# Supplementary material for: Fighting Selection Bias in Statistical Learning: Application to Visual Recognition from Biased Image Databases
Source: arXiv:2109.02357 source file (2022-11-01)
Supplement: Supplementary file 1 [file appendix.tex]

\subsection{Experimental details}

In \cref{tab:details-number-datasets}, we provide information about
the number recognition datasets involved in \cref{subsec:exp-number-reco}.
Precisely, we give the original size of the images as well as their
repartition over the numbers between 0 and 9.

In \cref{fig:num_obs_per_class_ms1m}, we provide information about the number
of observations per class (identity) in the MS1M dataset.

\newpage
\begin{table}
    \centering
    \footnotesize
    \begin{tabular}[t]{lccccc}
	\toprule
	& MNIST & notMNIST* & SynthDigits & MNIST-M & SVHN$^\star$ \\
	\midrule
	\# Obs & 70,000 & 18,724 & 19,106 & 68,002 &  99,289 \\
	$W\times H \times C$ & $28 \times 28\times 1$  & $28\times 28\times 1$ & 
	$32 \times 32\times 3$  & $32\times 32\times 3$ & $32 \times 32\times 3$ \\
	Number 0 (A)  & 6,903 & 1,872 & 1,900 & 6.703 & 6,692 \\
	Number 1 (B)  & 7,877 & 1,873 & 1,936 & 7,656 & 18,960 \\
	Number 2 (C)  & 6,990 & 1,873 & 1,842 & 6,786 & 14,734 \\
	Number 3 (D)  & 7,141 & 1,873 & 1,766 & 6,936 & 11,379 \\
	Number 4 (E)  & 6,824 & 1,873 & 1,878 & 6,636 & 9,981 \\
	Number 5 (F)  & 6,313 & 1,872 & 1,910 & 6,138 & 9,266 \\
	Number 6 (G)  & 6,876 & 1,872 & 2,032 & 6,668 & 7,704 \\
	Number 7 (H)  & 7,293 & 1,872 & 1,984 & 7,072 & 7,614 \\
	Number 8 (I)  & 6,825 & 1,872 & 1,958 & 6,637 & 6,705 \\
	Number 9 (J)  & 6,958 & 1,872 & 1,900 & 6,770 & 6,254 \\
	\bottomrule
    \end{tabular}
    \caption{Number of observations and original dimensions
    of the number/character recognition databases.\\
    *The classes in notMNIST correspond to the characters in parenthesis.\\
    $^\star$The class 10 of the original SVHN dataset is considered as 0 here.
    }\label{tab:details-number-datasets}
\end{table}

\begin{figure}[t]
    \centering
    \includegraphics[width=0.4\linewidth]{figures/face_exps/obs_per_class.pdf}
    \caption{Number of observations per class in the MS1M dataset.}
    \label{fig:num_obs_per_class_ms1m}
\end{figure}

\subsection{Robin notes}

Notations Laforgue, with the scenario in \cref{subsec:exp:est_bias},
assuming constant $p_{\text{test}}(y) = 1/Q$,
\begin{align*}
    \E_P\left[ \omega_k(Z) \omega_l(Z) \right]
    &= \E_P\left[ \Omega_k \cdot \frac{p_k(Y) }{p_{\text{test}}(Y)}
    \Omega_l \cdot \frac{p_l(Y) }{p_{\text{test}}(Y)} \right],\\
    &= \sum_{y \in \mathcal{Y}} 
    \Omega_k \Omega_l \cdot \frac{p_k(y) \cdot p_l(y) }{p_{\text{test}}(y)} ,\\
    &= Q \sum_{y \in \mathcal{Y}} 
    \Omega_k \Omega_l \cdot p_k(y) \cdot p_l(y)  ,\\
\end{align*}
\begin{align*}
    \Omega_k = \int \omega_k (z) p_{\text{test}}(z) \; dz
    = \frac{1}{Q} \sum_{y \in \mathcal{Y}} \omega_k (y).
\end{align*}
